# Supplementary material for: NeuralPCI: Spatio-temporal Neural Field for 3D Point Cloud Multi-frame Non-linear Interpolation
Source: arXiv:2303.15126 source file (2023-03-27)
Supplement: Supplementary file 1 [file dataset.tex]

\begin{table}[t]
\centering
\caption{\textbf{Overview of NL-Drive dataset.} Dataset split for train/val/test and proportion of each open-source dataset in the NL-Drive dataset.}
\label{table: dataset}
\scalebox{0.8}{
\begin{tabular}{ccccccccc}
\hline
\multirow{2}{*}{} & \multicolumn{4}{c}{\textbf{Number of Scenes}} & \multicolumn{4}{c}{\textbf{Number of Samples}}  \\ 
\cline{2-9}
                  & KITTI & Argos & Nuscenes & total & KITTI & Argos & Nuscenes & total      \\ 
\hline
Train             & 7     & 605    & 455   & 1067        & 1516     & 1508   & 1304  & 4328       \\
Val               & 2     & 123    & 60    & 185         & 308      & 355    & 305   & 968        \\
Test              & 2     & 124    & 169   & 295         & 311      & 311    & 303   & 925        \\
\hline
\end{tabular}}
\end{table}
