# Supplementary material for: NeuralPCI: Spatio-temporal Neural Field for 3D Point Cloud Multi-frame Non-linear Interpolation
Source: arXiv:2303.15126 source file (2023-03-27)
Supplement: Supplementary file 2 [file dynamic.tex]

\begin{table}
\centering
\caption{\textbf{Quantitative comparison for static and dynamic scenes. }}
\label{tab: dynamic}
\scalebox{0.95}{
\begin{tabular}{ccccccc} 
\hline
\multirow{2}{*}{Methods} & \multicolumn{2}{c}{Static} & \multicolumn{2}{c}{Dynamic} & \multicolumn{2}{c}{Overall}  \\ 
\cline{2-7}
 & CD & EMD & CD & EMD & CD & EMD \\ 
\hline
NSFP & 0.00 & 000.00 & 0.00 & 000.00 & 1.75 & 132.13 \\
PV-RAFT & 0.00 & 000.00 & 0.00 & 000.00  & 1.64 & 140.42 \\
PointINet & 0.00 & 000.00 & 0.00 & 000.00 & 1.06 & 101.12 \\
NeuralPCI & 0.00 & 000.00 & 0.00 & 000.00 & 0.80 & 97.03 \\
\hline
\end{tabular}}
\end{table}
