# Supplementary material for: NeuralPCI: Spatio-temporal Neural Field for 3D Point Cloud Multi-frame Non-linear Interpolation
Source: arXiv:2303.15126 source file (2023-03-27)
Supplement: Supplementary file 3 [file pt.tex]

\begin{table*}[htb]
\centering
\caption{\textbf{Quantitative comparison for diverse point cloud densities. }}
\label{tab:point cloud density}
\scalebox{0.95}{
\begin{tabular}{ccccccccccc} 
\hline
\multirow{2}{*}{Methods} & \multicolumn{2}{c}{1024pt} & \multicolumn{2}{c}{2048pt} & \multicolumn{2}{c}{4096pt} & \multicolumn{2}{c}{8192pt} & \multicolumn{2}{c}{16384pt}  \\ 
\cline{2-11}
     & CD & EMD & CD & EMD & CD & EMD & CD & EMD & CD & EMD \\
\hline
NSFP & 6.82 & 209.23 & 4.01 & 173.84 & 2.55 & 149.38 & 1.75 & 132.13 & 1.27 & 119.51 \\
PV-RAFT & 6.90 & 228.01 & 3.95 & 186.05 & 2.42 & 157.38 & 1.64 & 140.42 & 1.24 & 132.33 \\
PointINet & 5.68 & 193.28 & 3.08 & 153.72 & 1.74 & 123.27 & 1.06 & 101.12 & 0.71 & 85.20 \\
NeuralPCI& \textbf{5.03} & \textbf{185.20} & \textbf{2.58} & \textbf{146.94} & \textbf{1.36} & \textbf{119.03} & \textbf{0.80} & \textbf{97.03} & \textbf{0.45} & \textbf{84.35} \\
\hline
\end{tabular}}
\end{table*}
